# Supplementary material for: Evaluating Communicative Success in Machine-Translated Conversation
Source: arXiv:2609.19885 source file (2026-12-02)
Supplement: Supplementary file 1 [file appendix_judge_certainty.tex]

\begin{table}[htbp]
  \centering
  \caption{Naive vs.\ Rogan--Gladen-corrected accuracy for the Gemini judge. The naive CI is a
  plain Wilson interval and ignores judge error, while the corrected CI ($\approx4\times$ wider for the
  two baselines) accounts for calibration uncertainty too. $^\dagger$The frontier's correction
  saturates at 1.000 in 10 of 12 directions, a proxy-gold ceiling artifact, not a literal 100\%
  accuracy claim.}
  \label{tab:appendix-judge-certainty}
  \small
  \resizebox{\ifdim\width>\linewidth\linewidth\else\width\fi}{!}{%
  \begin{tabular}{@{}lcccc@{}}
    \toprule
    \textbf{Model} & \textbf{Naive $\hat p$} & \textbf{Naive 95\% CI} & \textbf{Corrected $\hat\theta$} & \textbf{Corrected 95\% CI} \\
    \midrule
    Gemini 3.1 Pro (frontier) & 0.897 & [0.896, 0.899] & 1.000$^\dagger$ & [1.000, 1.000]$^\dagger$ \\
    Gemini 3.1 Flash Lite & 0.767 & [0.765, 0.770] & 0.871 & [0.862, 0.880] \\
    Qwen3.5 Flash & 0.764 & [0.762, 0.767] & 0.867 & [0.859, 0.876] \\
    \bottomrule
  \end{tabular}}
\end{table}
